# Supplementary material for: Discrete Variational Attention Models for Language Generation
Source: arXiv:2004.09764 source file (2021-06-16)
Supplement: Supplementary file 1 [file appendix.tex]

\section{The network architecture for PixelCNN}
